# Supplementary material for: Selected Configuration Interaction for Resonances
Source: arXiv:2407.08576 source file (2024-08-08)
Supplement: Supplementary file 1 [file supp_inf_cap_cipsi.pdf]

# Supporting Information for "Selected Configuration Interaction for Resonances"

Yann Damour,[1, a)] Anthony Scemama,[1] Fábris Kossoski,[1, b)] and Pierre-François Loos[1, c)]
*Laboratoire de Chimie et Physique Quantiques (UMR 5626), Université de Toulouse, CNRS, UPS, France*

## S1. ADDITIONAL BASIS SET FUNCTIONS

### A. $N_2$

```
Angular momentum    Exponent      Coefficient
S                   0.0288000     1.0
S                   0.0144000     1.0
S                   0.0072000     1.0
P                   0.0245500     1.0
P                   0.0122750     1.0
P                   0.0061375     1.0
D                   0.0755000     1.0
D                   0.0377500     1.0
D                   0.0188750     1.0
```

### B. CO

```
Angular momentum    Exponent      Coefficient
S                   0.029445000   1.0
S                   0.014722500   1.0
S                   0.007361250   1.0
P                   0.023857500   1.0
P                   0.011928750   1.0
P                   0.005964375   1.0
D                   0.078500000   1.0
D                   0.039250000   1.0
D                   0.019625000   1.0
```

## S2. HARTREE FOCK AND EXTENDED CIS ENERGIES

TABLE S1: Hartree-Fock ($E_{\text{HF}}$), extended CIS ($E_{\text{XCIS}}$) and extended CAP-CIS ($E_{\text{CAP-XCIS}}$) energies, in Hartree, for the neutral and anionic states of $N_2$ and CO in the aug-cc-pVTZ+3s3p3d basis set.

| | | | $E_{\text{CAP-XCIS}}$ | |
|---|---|---|---|---|
| | $E_{\text{HF}}$ | $E_{\text{XCIS}}$ | Re | Im |
| $N_2$ | −108.9848674642 | | | |
| $N_2^-$ | −108.9730322329 | −108.8659914433 | −108.8673661907 | −0.0240118798 |
| CO | −112.7815840103 | | | |
| $CO^-$ | −112.7706126698 | −112.6573186010 | −112.6708127100 | −0.0274768495 |

a)Electronic mail: yann.damour@irsamc.ups-tlse.fr
b)Electronic mail: fabris.kossoski@irsamc.ups-tlse.fr
c)Electronic mail: loos@irsamc.ups-tlse.fr

## S3. $N_2$

TABLE S2: Extrapolated total energy ($E_{\mathrm{exFCI}}$) and first-order corrected total energy ($\tilde{E}_{\mathrm{exFCI}}$), in Hartree, for the ground state of $N_2$ computed with NON orbitals in the aug-cc-pVTZ+3s3p3d basis set.

| | $E_{\mathrm{exFCI}}$ | | $\tilde{E}_{\mathrm{exFCI}}$ | |
|---|---|---|---|---|
| # of fitting points | Re | Im | Re | Im |
| 3 | −109.4137(2) | −0.000098(3) | −109.4137(2) | −0.00000068(7) |
| 4 | −109.41379(2) | −0.0000976(3) | −109.41370(2) | −0.0000007(2) |
| 5 | −109.41369(2) | −0.0000976(1) | −109.41369(2) | −0.00000065(5) |

## S4. $N_2^-$

### A. Influence of the orbital set

TABLE S3: Extrapolated total energy ($E_{\text{exFCI}}$), in Hartree, for the $^2\Pi_g$ shape resonance of $N_2^-$ in the aug-cc-pVTZ+3s3p3d basis set. Four sets of orbitals are considered: HFN, HFA, NON, and NOA (see main text for more details).

| | # of fitting points | $E_{\text{exFCI}}$ Re | $E_{\text{exFCI}}$ Im |
|---|---|---|---|
| HFN | 3 | −109.33(1) | −0.007(6) |
| | 4 | −109.326(2) | −0.007(1) |
| | 5 | −109.326(2) | −0.006(2) |
| HFA | 3 | −109.3249(3) | −0.007(4) |
| | 4 | −109.325(1) | −0.007(1) |
| | 5 | −109.325(1) | −0.007(1) |
| NON | 3 | −109.324(8) | −0.007(1) |
| | 4 | −109.324(1) | −0.0072(4) |
| | 5 | −109.3240(4) | −0.007(1) |
| NOA | 3 | −109.3237(4) | −0.0073(2) |
| | 4 | −109.32370(3) | −0.00728(6) |
| | 5 | −109.32369(3) | −0.00728(2) |

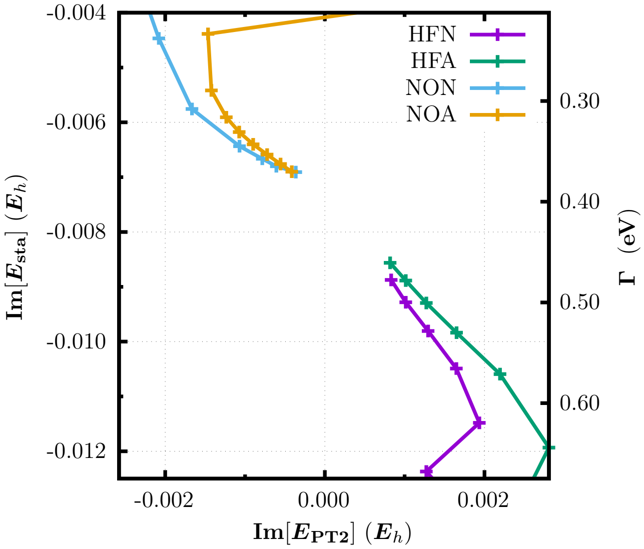


FIG. S1: Evolution of the imaginary part of the CAP-CIPSI energy as a function of the imaginary part of the second-order energy correction Im[$E_{\text{PT2}}$], for the $^2\Pi_g$ shape resonance of $N_2^-$ in the aug-cc-pVTZ+3s3p3d basis set. Four different sets of orbitals are considered: HFN, HFA, NON, and NOA (see main text for more details). Resonance position $E_R$ and width $\Gamma$ are obtained for the fixed extrapolated energy of the neutral system.

### B. Influence of the selection criterion

TABLE S4: Extrapolated total energy ($E_{\text{exFCI}}$), in Hartree, for the $^2\Pi_g$ shape resonance of $N_2{}^-$ in the aug-cc-pVTZ+3s3p3d basis set. Three selection criteria are considered: $|e_\alpha^{(2)}|$, $\text{Re}[e_\alpha^{(2)}]$, and $\text{Im}[e_\alpha^{(2)}]$ (see main text for more details).

| | # of fitting points | $E_{\text{exFCI}}$ Re | $E_{\text{exFCI}}$ Im |
|---|---|---|---|
| | 3 | −109.3237(4) | −0.0073(2) |
| $\left\|e_\alpha^{(2)}\right\|$ | 4 | −109.32370(3) | −0.00728(6) |
| | 5 | −109.32369(3) | −0.00728(2) |
| | 3 | −109.324(1) | −0.006(2) |
| $\text{Re}[e_\alpha^{(2)}]$ | 4 | −109.3240(2) | −0.0063(7) |
| | 5 | −109.3240(1) | −0.0063(3) |
| | 3 | −109.3237(9) | −0.0073(5) |
| $\text{Im}[e_\alpha^{(2)}]$ | 4 | −109.32374(8) | −0.00729(4) |
| | 5 | −109.32374(4) | −0.00729(2) |

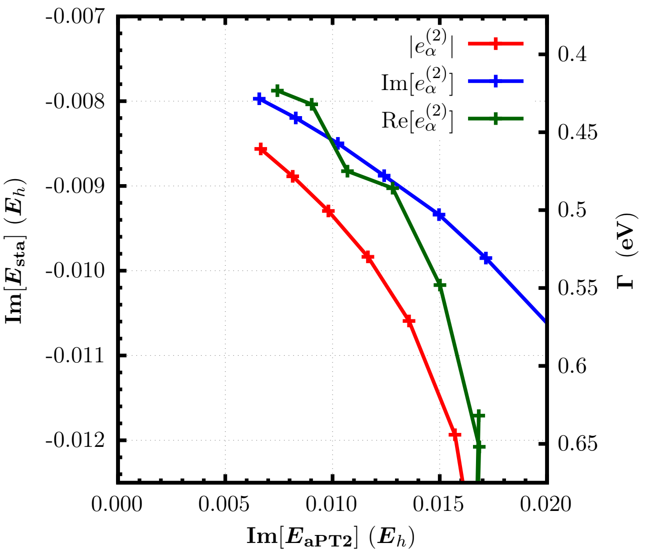


FIG. S2: Evolution of the imaginary part of the CAP-CIPSI energy as a function of the imaginary part of the second-order energy correction $\text{Im}[E_{\text{aPT2}}]$, for the $^2\Pi_g$ shape resonance of $N_2{}^-$ with HFA orbitals in the aug-cc-pVTZ+3s3p3d basis set. Three selection criteria are considered: $|e_\alpha^{(2)}|$, $\text{Re}[e_\alpha^{(2)}]$, and $\text{Im}[e_\alpha^{(2)}]$ (see main text for more details). Resonance position $E_R$ and width $\Gamma$ are obtained for the fixed extrapolated energy of the neutral system.

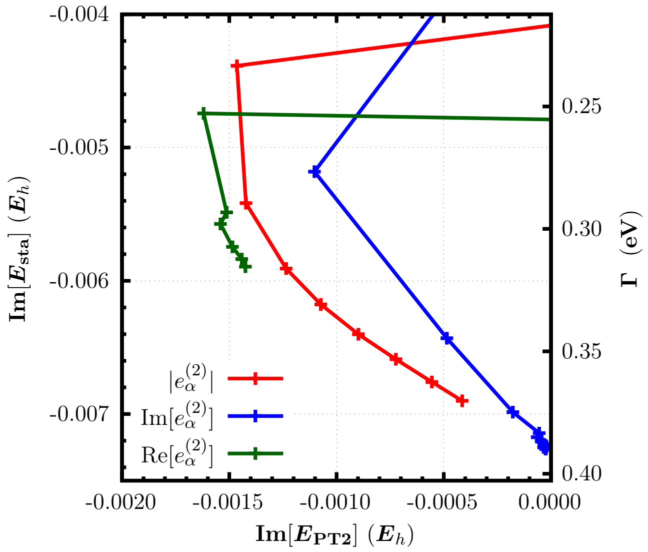


FIG. S3: Evolution of the imaginary part of the CAP-CIPSI energy as a function of the imaginary part of the second-order energy correction Im[$E_{\mathrm{PT2}}$], for the $^2\Pi_g$ shape resonance of ${N_2}^-$ with NOA orbitals in the aug-cc-pVTZ+3s3p3d basis set. Three selection criteria are considered: $|e_\alpha^{(2)}|$, Re[$e_\alpha^{(2)}$], and Im[$e_\alpha^{(2)}$] (see main text for more details). Resonance position $E_R$ and width Γ are obtained for the fixed extrapolated energy of the neutral system.

### C. First-order corrected energy

TABLE S5: Extrapolated first-order corrected total energy ($\tilde{E}_{\text{exFCI}}$), in Hartree, for the $^2\Pi_g$ shape resonance of $N_2{}^-$ computed with NOA orbitals in the aug-cc-pVTZ+3s3p3d basis set.

| # of fitting points | $\tilde{E}_{\text{exFCI}}$ Re | Im |
|---|---|---|
| 3 | −109.3242(7) | −0.006(1) |
| 4 | −109.3242(2) | −0.0056(3) |
| 5 | −109.3242(1) | −0.0057(3) |

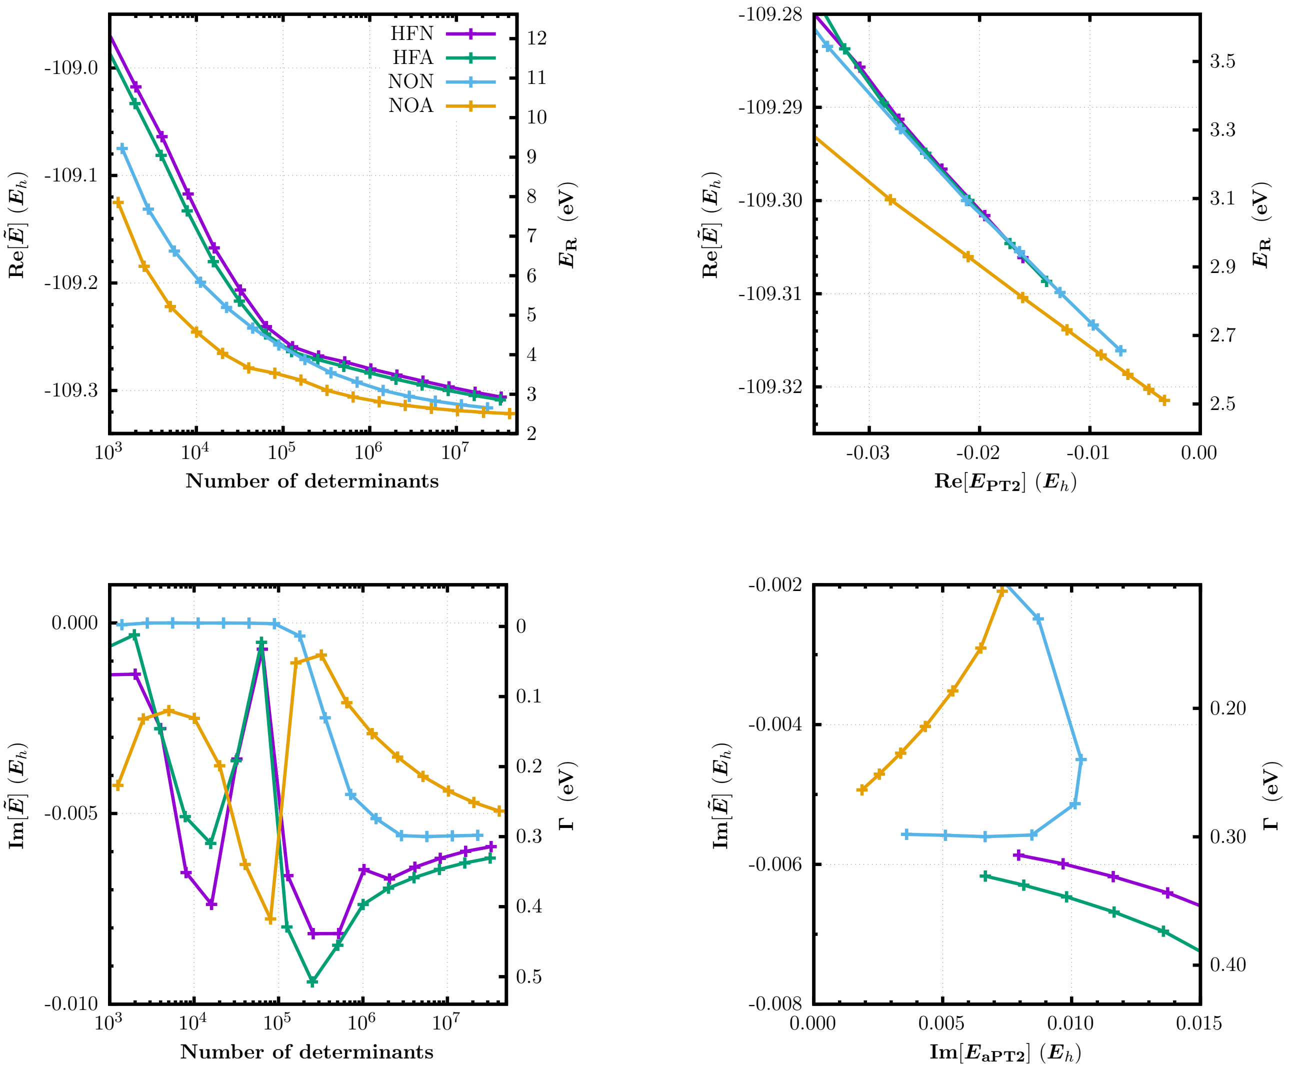


FIG. S4: Evolution of the real and imaginary part of the first-order corrected CAP-CIPSI energy, for the $^2\Pi_g$ shape resonance of $N_2{}^-$ in the aug-cc-pVTZ+3s3p3d basis set, as functions of the number of determinants and second-order energy correction. Four different sets of orbitals are considered: HFN, HFA, NON, and NOA (see main text for more details). Resonance position $E_R$ and width $\Gamma$ are obtained for the fixed extrapolated energy of the neutral system.

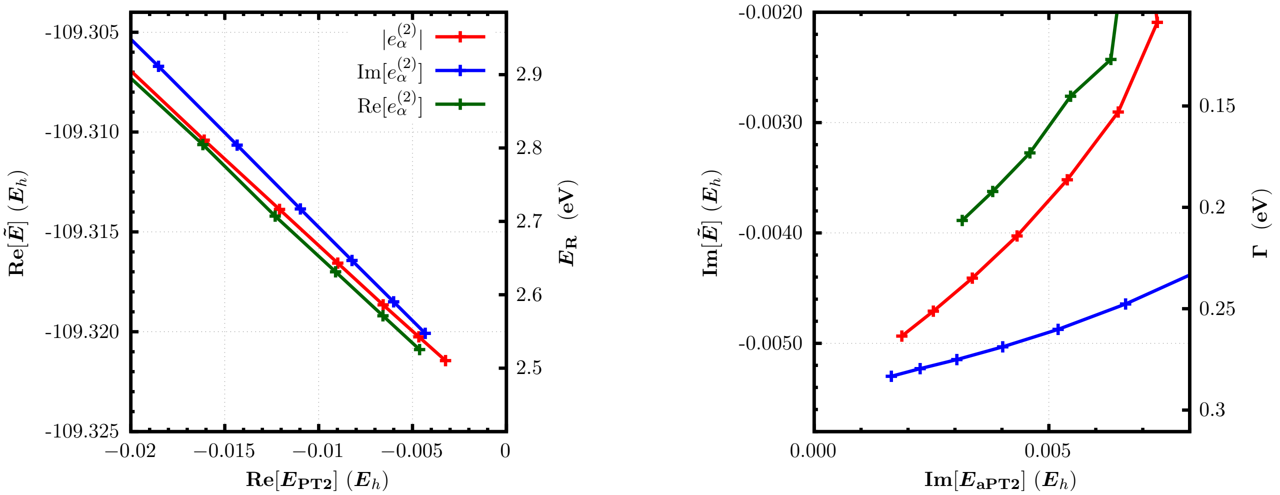


FIG. S5: Evolution of the real and imaginary part of the first-order corrected CAP-CIPSI energy, for the $^2\Pi_g$ shape resonance of $N_2{}^-$ in the aug-cc-pVTZ+3s3p3d basis set, as functions of the second-order energy correction. Three selection criteria are considered: $|e_\alpha^{(2)}|$, $\mathrm{Re}[e_\alpha^{(2)}]$ and $\mathrm{Im}[e_\alpha^{(2)}]$ (see main text for more details). Resonance position $E_R$ and width $\Gamma$ are obtained for the fixed extrapolated energy of the neutral system.

## S5. CO

TABLE S6: Extrapolated total energy ($E_{\mathrm{exFCI}}$) and first-order corrected energy ($\tilde{E}_{\mathrm{exFCI}}$), in Hartree, for the ground state of CO computed with NON orbitals in the aug-cc-pVTZ+3s3p3d basis set.

| | $E_{\mathrm{exFCI}}$ | | $\tilde{E}_{\mathrm{exFCI}}$ | |
|---|---|---|---|---|
| # of fitting points | Re | Im | Re | Im |
| 3 | −113.1938(6) | −0.00022(1) | −113.1938(6) | −0.000001(2) |
| 4 | −113.19376(6) | −0.000218(2) | −113.19376(6) | −0.0000007(2) |
| 5 | −113.19375(3) | −0.0002177(7) | −113.19376(3) | −0.0000007(1) |

## S6. $CO^-$

TABLE S7: Extrapolated total energy ($E_{\text{exFCI}}$) and first-order corrected total energy ($\tilde{E}_{\text{exFCI}}$), in Hartree, for the $^2\Pi$ shape resonance of $CO^-$ computed with NOA orbitals in the aug-cc-pVTZ+3s3p3d basis set.

| | $E_{\text{exFCI}}$ | | $\tilde{E}_{\text{exFCI}}$ | |
|---|---|---|---|---|
| # of fitting points | Re | Im | Re | Im |
| 3 | −113.118(3) | −0.011(1) | −113.119(2) | −0.013(2) |
| 4 | −113.1180(3) | −0.0114(3) | −113.1189(5) | −0.0128(2) |
| 5 | −113.1180(2) | −0.0114(1) | −113.1188(3) | −0.0130(8) |

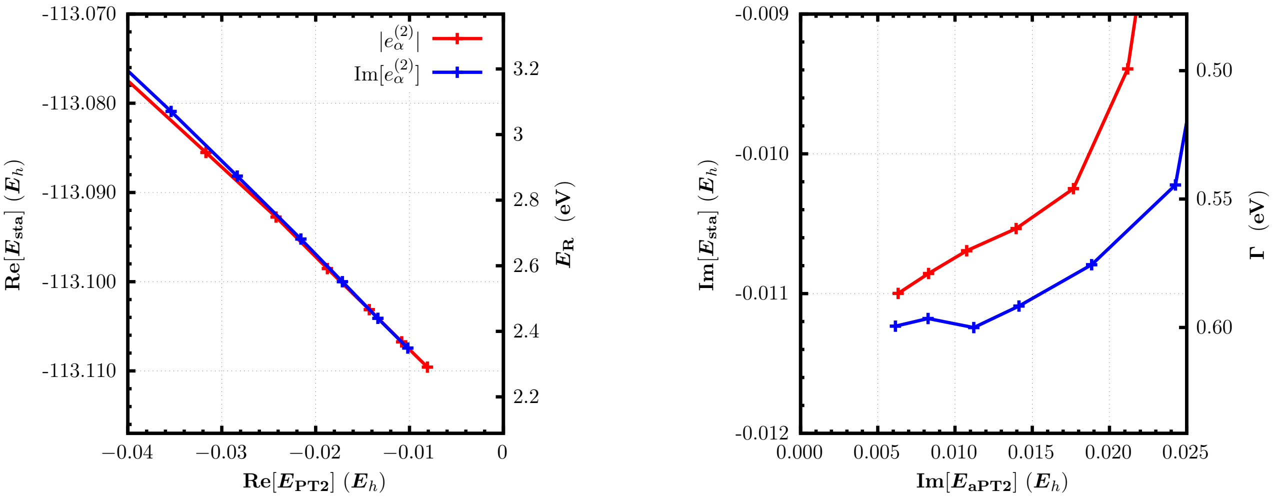


FIG. S6: Evolution of the real and imaginary parts of the total CAP-CIPSI energy as functions of the second-order energy correction for the $^2\Pi$ shape resonance of $CO^-$ computed in the aug-cc-pVTZ+3s3p3d basis set for the three selection criteria described in the main text and NOA. Resonance position $E_R$ and width $\Gamma$ are obtained for the fixed extrapolated energy of the neutral system.

## S7. EXTRAPOLATION PROCEDURE

To generate the CAP-exFCI estimates, extrapolations of the CAP-CIPSI stationary energy as a function of the second-order energy are performed using weighted linear fits on the values corresponding to the $M$ latest CAP-CIPSI iterations. The uncertainties associated with the CAP-exFCI values are expressed as a confidence interval from the standard error of the intercept $\mathrm{SE}_{\text{CAP-exFCI}}$ given by the fit and a $t$-multiplier $t^*_{M-2}$ corresponding to a 99%-confidence interval. The standard error of the intercept is

$$\mathrm{SE}_{\text{CAP-exFCI}} = \sqrt{\frac{\sum_{m=1}^{M} w_m (y_m - \hat{y}_m)^2}{M-2} \left( \boldsymbol{X}^T \cdot \boldsymbol{W} \cdot \boldsymbol{X} \right)^{-1}_{1,1}} \tag{S1}$$

where $M$ is the number of fitting points, $w_m$ is the inverse of the square of the second-order energy corresponding to the $m$th point, $y_m$ is the calculated stationary energy of the $m$th point, $\hat{y}_m$ is the energy of the $m$th point given by the linear fit, $\boldsymbol{W}$ is a diagonal matrix built from $\{w_m\}_{m=1}^{M}$ and $\boldsymbol{X}$ is the matrix

$$\boldsymbol{X} = \begin{pmatrix} 1 & x_1 \\ 1 & x_2 \\ \vdots & \vdots \\ 1 & x_M \end{pmatrix} \tag{S2}$$

in which $x_m$ is the second-order energy of the $m$th point. Thus, the resulting uncertainty is

$$E_{\text{CAP-exFCI}} \pm t^*_{M-2} \mathrm{SE}_{\text{CAP-exFCI}} \tag{S3}$$
