# Supplementary material for: Selected Configuration Interaction for Resonances
Source: arXiv:2407.08576 ancillary file (2024-08-08)
Supplement: Supplementary file 2 [file supp_inf_cap_cipsi.pdf]

# Supporting Information for “Selected Configuration Interaction for Resonances”

Yann Damour\*, Anthony Scemama, F  bris Kossoski\*, and Pierre-Fran  ois Loos\*

*Laboratoire de Chimie et Physique Quantiques (UMR 5626), Universit   de Toulouse, CNRS, UPS, 31062 Toulouse, France*

## S1. ADDITIONAL BASIS SET FUNCTIONS

### A. N<sub>2</sub>

| Angular momentum | Exponent  | Coefficient |
|------------------|-----------|-------------|
| S                | 0.0288000 | 1.0         |
| S                | 0.0144000 | 1.0         |
| S                | 0.0072000 | 1.0         |
| P                | 0.0245500 | 1.0         |
| P                | 0.0122750 | 1.0         |
| P                | 0.0061375 | 1.0         |
| D                | 0.0755000 | 1.0         |
| D                | 0.0377500 | 1.0         |
| D                | 0.0188750 | 1.0         |

### B. CO

| Angular momentum | Exponent    | Coefficient |
|------------------|-------------|-------------|
| S                | 0.029445000 | 1.0         |
| S                | 0.014722500 | 1.0         |
| S                | 0.007361250 | 1.0         |
| P                | 0.023857500 | 1.0         |
| P                | 0.011928750 | 1.0         |
| P                | 0.005964375 | 1.0         |
| D                | 0.078500000 | 1.0         |
| D                | 0.039250000 | 1.0         |
| D                | 0.019625000 | 1.0         |

## S2. HARTREE FOCK AND EXTENDED CIS ENERGIES

TABLE S1: Hartree-Fock ( $E_{\text{HF}}$ ), extended CIS ( $E_{\text{XCIS}}$ ) and extended CAP-CIS ( $E_{\text{CAP-XCIS}}$ ) energies, in Hartree, for the neutral and anionic states of N<sub>2</sub> and CO in the aug-cc-pVTZ+3s3p3d basis set.

|                             | $E_{\text{HF}}$ | $E_{\text{XCIS}}$ | $E_{\text{CAP-XCIS}}$ |               |
|-----------------------------|-----------------|-------------------|-----------------------|---------------|
|                             |                 |                   | Re                    | Im            |
| N <sub>2</sub>              | −108.9848674642 |                   |                       |               |
| N <sub>2</sub> <sup>−</sup> | −108.9730322329 | −108.8659914433   | −108.8673661907       | −0.0240118798 |
| CO                          | −112.7815840103 |                   |                       |               |
| CO <sup>−</sup>             | −112.7706126698 | −112.6573186010   | −112.6708127100       | −0.0274768495 |

S3. N<sub>2</sub>

TABLE S2: Extrapolated total energy ( $E_{\text{exFCI}}$ ) and first-order corrected total energy ( $\tilde{E}_{\text{exFCI}}$ ), in Hartree, for the ground state of N<sub>2</sub> computed with NON orbitals in the aug-cc-pVTZ+3s3p3d basis set.

| # of fitting points | $E_{\text{exFCI}}$ |               | $\tilde{E}_{\text{exFCI}}$ |                |
|---------------------|--------------------|---------------|----------------------------|----------------|
|                     | Re                 | Im            | Re                         | Im             |
| 3                   | -109.4137(2)       | -0.000098(3)  | -109.4137(2)               | -0.00000068(7) |
| 4                   | -109.41379(2)      | -0.0000976(3) | -109.41370(2)              | -0.0000007(2)  |
| 5                   | -109.41369(2)      | -0.0000976(1) | -109.41369(2)              | -0.00000065(5) |

S4.  $\text{N}_2^-$ 

## A. Influence of the orbital set

TABLE S3: Extrapolated total energy ( $E_{\text{exFCI}}$ ), in Hartree, for the  $^2\Pi_g$  shape resonance of  $\text{N}_2^-$  in the aug-cc-pVTZ+3s3p3d basis set. Four sets of orbitals are considered: HFN, HFA, NON, and NOA (see main text for more details).

|     | # of fitting points | $E_{\text{exFCI}}$ |             |
|-----|---------------------|--------------------|-------------|
|     |                     | Re                 | Im          |
| HFN | 3                   | -109.33(1)         | -0.007(6)   |
|     | 4                   | -109.326(2)        | -0.007(1)   |
|     | 5                   | -109.326(2)        | -0.006(2)   |
| HFA | 3                   | -109.3249(3)       | -0.007(4)   |
|     | 4                   | -109.325(1)        | -0.007(1)   |
|     | 5                   | -109.325(1)        | -0.007(1)   |
| NON | 3                   | -109.324(8)        | -0.007(1)   |
|     | 4                   | -109.324(1)        | -0.0072(4)  |
|     | 5                   | -109.3240(4)       | -0.007(1)   |
| NOA | 3                   | -109.3237(4)       | -0.0073(2)  |
|     | 4                   | -109.32370(3)      | -0.00728(6) |
|     | 5                   | -109.32369(3)      | -0.00728(2) |

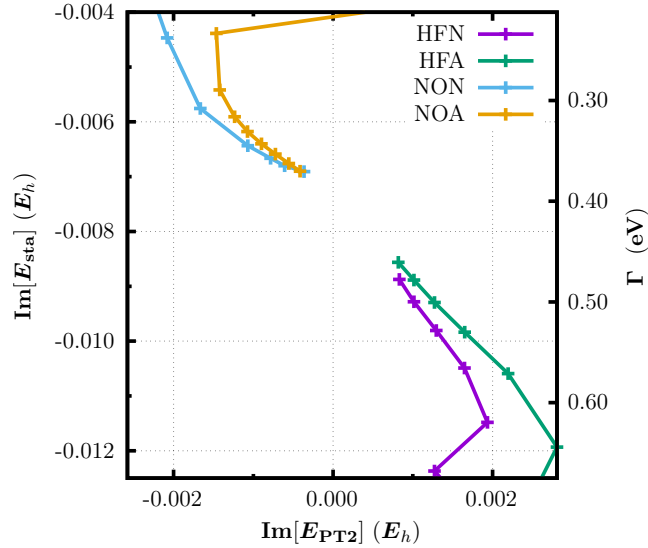

FIG. S1: Evolution of the imaginary part of the CAP-CIPSI energy as a function of the imaginary part of the second-order energy correction  $\text{Im}[E_{\text{PT2}}]$ , for the  $^2\Pi_g$  shape resonance of  $\text{N}_2^-$  in the aug-cc-pVTZ+3s3p3d basis set. Four different sets of orbitals are considered: HFN, HFA, NON, and NOA (see main text for more details). Resonance position  $E_R$  and width  $\Gamma$  are obtained for the fixed extrapolated energy of the neutral system.

### B. Influence of the selection criterion

TABLE S4: Extrapolated total energy ( $E_{\text{exFCI}}$ ), in Hartree, for the  $^2\Pi_g$  shape resonance of  $\text{N}_2^-$  in the aug-cc-pVTZ+3s3p3d basis set. Three selection criteria are considered:  $|e_\alpha^{(2)}|$ ,  $\text{Re}[e_\alpha^{(2)}]$ , and  $\text{Im}[e_\alpha^{(2)}]$  (see main text for more details).

|                             | # of fitting points | $E_{\text{exFCI}}$ |             |
|-----------------------------|---------------------|--------------------|-------------|
|                             |                     | Re                 | Im          |
| $ e_\alpha^{(2)} $          | 3                   | -109.3237(4)       | -0.0073(2)  |
|                             | 4                   | -109.32370(3)      | -0.00728(6) |
|                             | 5                   | -109.32369(3)      | -0.00728(2) |
| $\text{Re}[e_\alpha^{(2)}]$ | 3                   | -109.324(1)        | -0.006(2)   |
|                             | 4                   | -109.3240(2)       | -0.0063(7)  |
|                             | 5                   | -109.3240(1)       | -0.0063(3)  |
| $\text{Im}[e_\alpha^{(2)}]$ | 3                   | -109.3237(9)       | -0.0073(5)  |
|                             | 4                   | -109.32374(8)      | -0.00729(4) |
|                             | 5                   | -109.32374(4)      | -0.00729(2) |

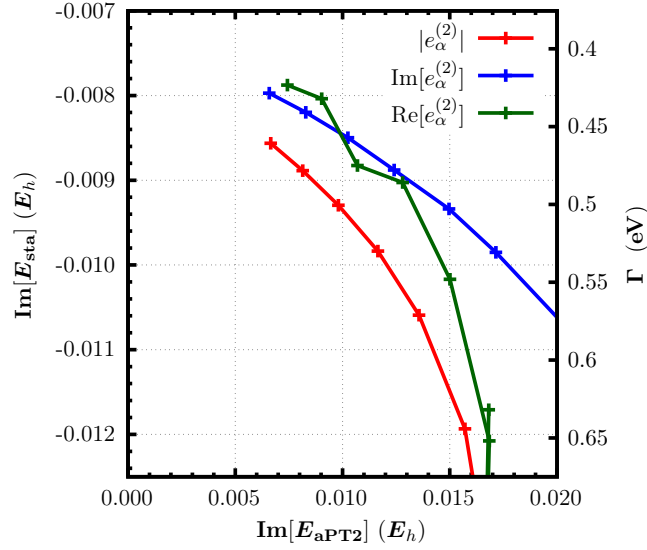

FIG. S2: Evolution of the imaginary part of the CAP-CIPSI energy as a function of the imaginary part of the second-order energy correction  $\text{Im}[E_{\text{aPT2}}]$ , for the  $^2\Pi_g$  shape resonance of  $\text{N}_2^-$  with HFA orbitals in the aug-cc-pVTZ+3s3p3d basis set. Three selection criteria are considered:  $|e_\alpha^{(2)}|$ ,  $\text{Re}[e_\alpha^{(2)}]$ , and  $\text{Im}[e_\alpha^{(2)}]$  (see main text for more details). Resonance position  $E_R$  and width  $\Gamma$  are obtained for the fixed extrapolated energy of the neutral system.

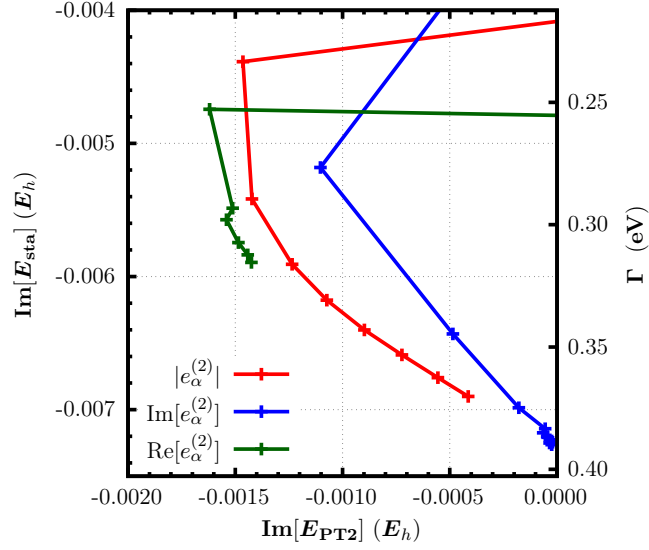

FIG. S3: Evolution of the imaginary part of the CAP-CIPSI energy as a function of the imaginary part of the second-order energy correction  $\text{Im}[E_{\text{PT2}}]$ , for the  $^2\Pi_g$  shape resonance of  $\text{N}_2^-$  with NOA orbitals in the aug-cc-pVTZ+3s3p3d basis set. Three selection criteria are considered:  $|e_\alpha^{(2)}|$ ,  $\text{Re}[e_\alpha^{(2)}]$ , and  $\text{Im}[e_\alpha^{(2)}]$  (see main text for more details). Resonance position  $E_R$  and width  $\Gamma$  are obtained for the fixed extrapolated energy of the neutral system.

### C. First-order corrected energy

TABLE S5: Extrapolated first-order corrected total energy ( $\tilde{E}_{\text{exFCI}}$ ), in Hartree, for the  $^2\Pi_g$  shape resonance of  $\text{N}_2^-$  computed with NOA orbitals in the aug-cc-pVTZ+3s3p3d basis set.

| # of fitting points | $\tilde{E}_{\text{exFCI}}$ |            |
|---------------------|----------------------------|------------|
|                     | Re                         | Im         |
| 3                   | -109.3242(7)               | -0.006(1)  |
| 4                   | -109.3242(2)               | -0.0056(3) |
| 5                   | -109.3242(1)               | -0.0057(3) |

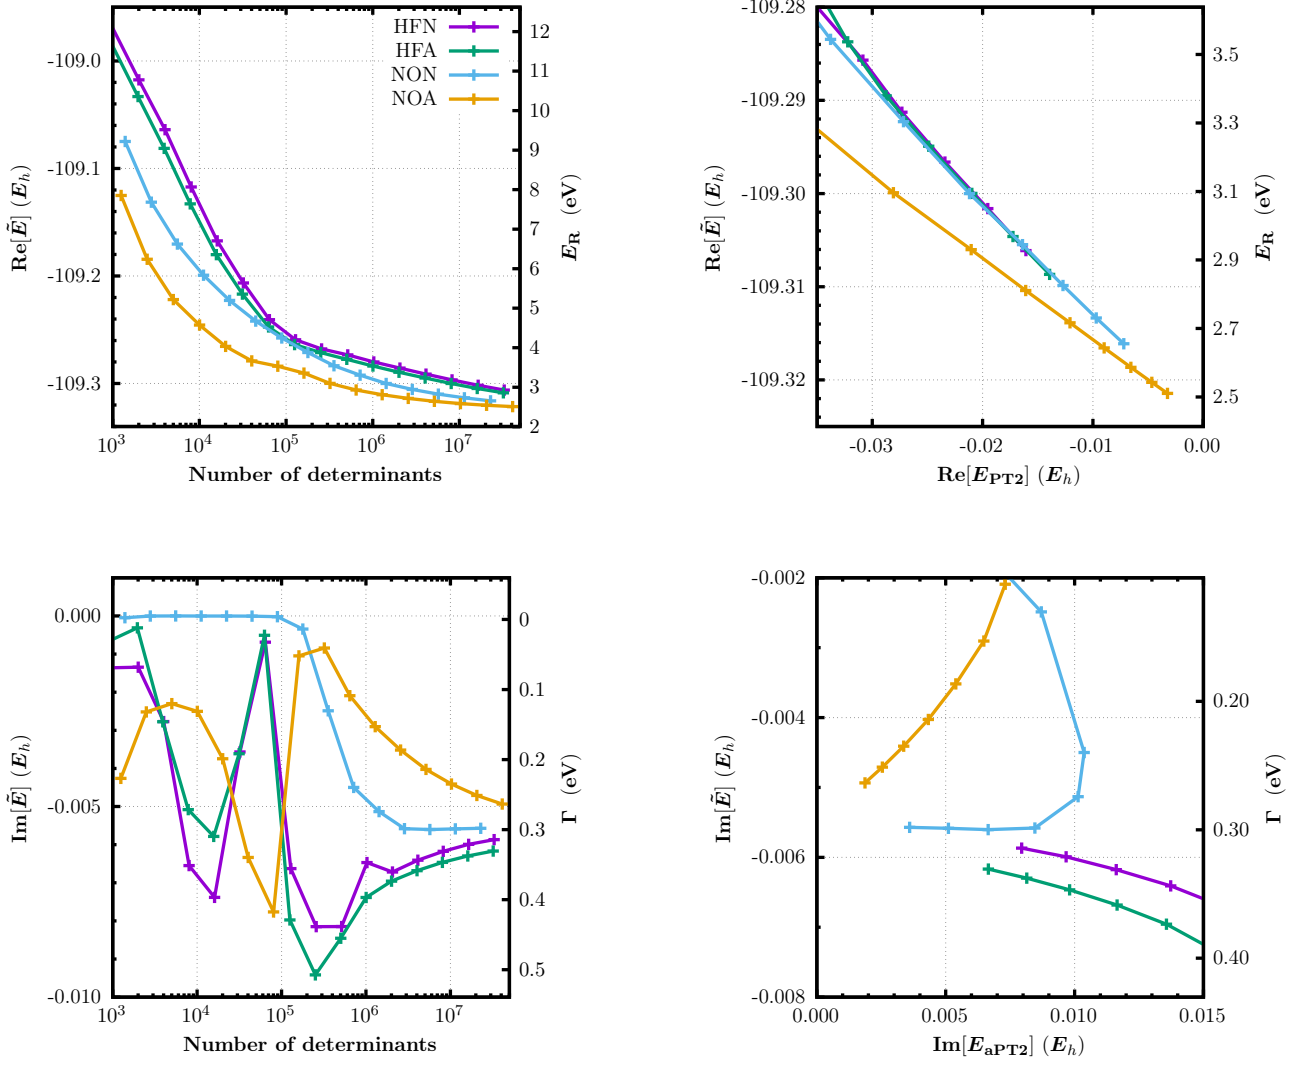

FIG. S4: Evolution of the real and imaginary part of the first-order corrected CAP-CIPSI energy, for the  $^2\Pi_g$  shape resonance of  $\text{N}_2^-$  in the aug-cc-pVTZ+3s3p3d basis set, as functions of the number of determinants and second-order energy correction. Four different sets of orbitals are considered: HFN, HFA, NON, and NOA (see main text for more details). Resonance position  $E_R$  and width  $\Gamma$  are obtained for the fixed extrapolated energy of the neutral system.

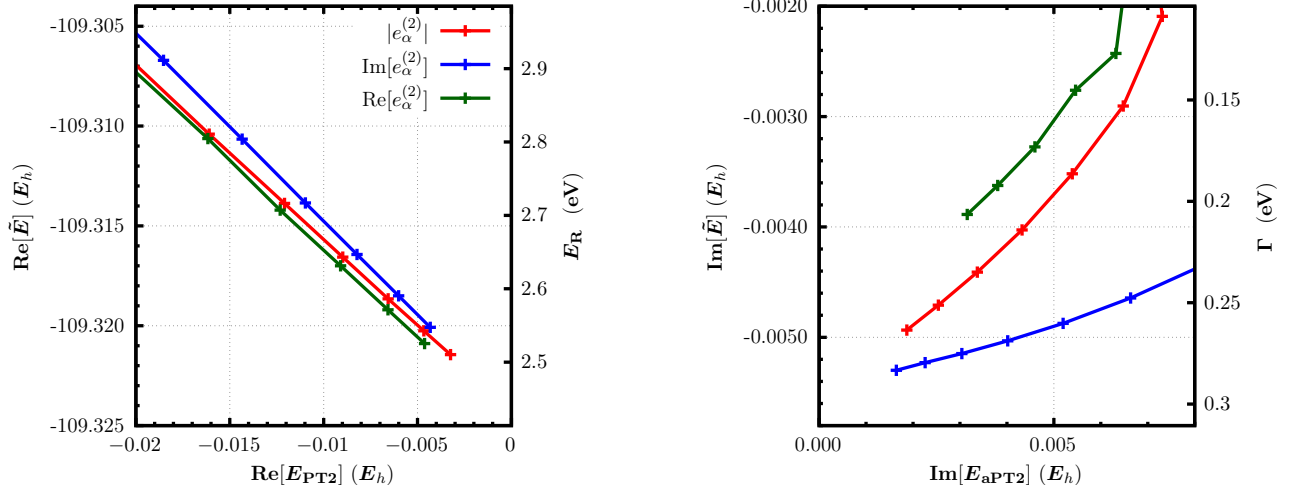

FIG. S5: Evolution of the real and imaginary part of the first-order corrected CAP-CIPSI energy, for the  $2\Pi_g$  shape resonance of  $\text{N}_2^-$  in the aug-cc-pVTZ+3s3p3d basis set, as functions of the second-order energy correction. Three selection criteria are considered:  $|e_\alpha^{(2)}|$ ,  $\text{Re}[e_\alpha^{(2)}]$  and  $\text{Im}[e_\alpha^{(2)}]$  (see main text for more details). Resonance position  $E_R$  and width  $\Gamma$  are obtained for the fixed extrapolated energy of the neutral system.

## S5. CO

TABLE S6: Extrapolated total energy ( $E_{\text{exFCI}}$ ) and first-order corrected energy ( $\tilde{E}_{\text{exFCI}}$ ), in Hartree, for the ground state of CO computed with NON orbitals in the aug-cc-pVTZ+3s3p3d basis set.

| # of fitting points | $E_{\text{exFCI}}$ |               | $\tilde{E}_{\text{exFCI}}$ |               |
|---------------------|--------------------|---------------|----------------------------|---------------|
|                     | Re                 | Im            | Re                         | Im            |
| 3                   | -113.1938(6)       | -0.00022(1)   | -113.1938(6)               | -0.000001(2)  |
| 4                   | -113.19376(6)      | -0.000218(2)  | -113.19376(6)              | -0.0000007(2) |
| 5                   | -113.19375(3)      | -0.0002177(7) | -113.19376(3)              | -0.0000007(1) |



S6.  $\text{CO}^-$ 

TABLE S7: Extrapolated total energy ( $E_{\text{exFCI}}$ ) and first-order corrected total energy ( $\tilde{E}_{\text{exFCI}}$ ), in Hartree, for the  $^2\Pi$  shape resonance of  $\text{CO}^-$  computed with NOA orbitals in the aug-cc-pVTZ+3s3p3d basis set.

| # of fitting points | $E_{\text{exFCI}}$ |             | $\tilde{E}_{\text{exFCI}}$ |             |
|---------------------|--------------------|-------------|----------------------------|-------------|
|                     | Re                 | Im          | Re                         | Im          |
| 3                   | -113.118(4)        | -0.0115(2)  | -113.119(1)                | -0.0128(7)  |
| 4                   | -113.1181(3)       | -0.01144(6) | -113.1190(1)               | -0.01279(9) |
| 5                   | -113.1180(2)       | -0.0114(1)  | -113.1190(2)               | -0.01280(8) |

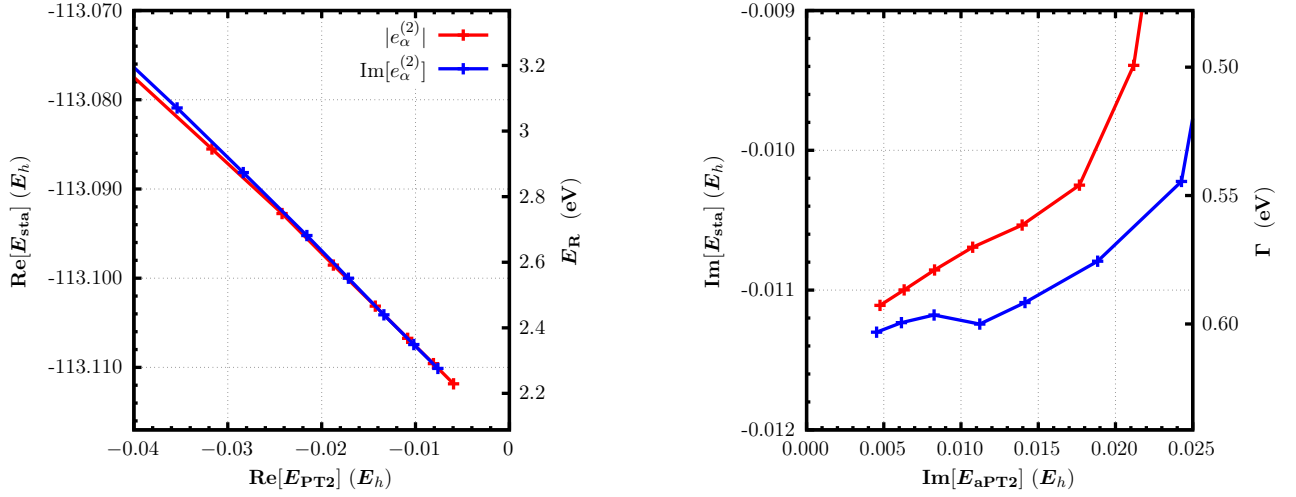

FIG. S6: Evolution of the real and imaginary parts of the total CAP-CIPSI energy as functions of the second-order energy correction for the  $^2\Pi$  shape resonance of  $\text{CO}^-$  computed in the aug-cc-pVTZ+3s3p3d basis set for the three selection criteria described in the main text and NOA. Resonance position  $E_R$  and width  $\Gamma$  are obtained for the fixed extrapolated energy of the neutral system.

### S7. EXTRAPOLATION PROCEDURE

To generate the CAP-exFCI estimates, extrapolations of the CAP-CIPSI stationary energy as a function of the second-order energy are performed using weighted linear fits on the values corresponding to the  $M$  latest CAP-CIPSI iterations. The uncertainties associated with the CAP-exFCI values are expressed as a confidence interval from the standard error of the intercept  $\text{SE}_{\text{CAP-exFCI}}$  given by the fit and a  $t$ -multiplier  $t_{M-2}^*$  corresponding to a 99%-confidence interval. The standard error of the intercept is

$$\text{SE}_{\text{CAP-exFCI}} = \sqrt{\frac{\sum_{m=1}^M w_m (y_m - \hat{y}_m)^2}{M-2} \left( \mathbf{X}^T \cdot \mathbf{W} \cdot \mathbf{X} \right)^{-1}_{1,1}} \quad (\text{S1})$$

where  $M$  is the number of fitting points,  $w_m$  is the inverse of the square of the second-order energy corresponding to the  $m$ th point,  $y_m$  is the calculated stationary energy of the  $m$ th point,  $\hat{y}_m$  is the energy of the  $m$ th point given by the linear fit,  $\mathbf{W}$  is a diagonal matrix built from  $\{w_m\}_{m=1}^M$  and  $\mathbf{X}$  is the matrix

$$\mathbf{X} = \begin{pmatrix} 1 & x_1 \\ 1 & x_2 \\ \vdots & \vdots \\ 1 & x_M \end{pmatrix} \quad (\text{S2})$$

in which  $x_m$  is the second-order energy of the  $m$ th point. Thus, the resulting uncertainty is

$$E_{\text{CAP-exFCI}} \pm t_{M-2}^* \text{SE}_{\text{CAP-exFCI}} \quad (\text{S3})$$
